# Supplementary material for: Diffusion as Shader: 3D-aware Video Diffusion for Versatile Video Generation Control
Source: arXiv:2501.03847 source file (2025-01-09)
Supplement: Supplementary file 1 [file X_appendix.tex]

\appendix
\section{Appendix}
